# Supplementary material for: Toward Planet-Wide Traffic Camera Calibration
Source: arXiv:2311.04243 source file (2023-11-06)
Supplement: Supplementary file 1 [file supp.tex]

\section{Summary and More Results}
For a thorough summary of our method and more results, \textbf{please see the video attached to the Supplementary Material.}

\section{Baselines Details}
In our main paper, we conducted a comprehensive comparison of our proposed method with several state-of-the-art (SOTA) automatic camera calibration approaches, specifically designed for traffic cameras. These methods include OptInOpt~\cite{bartl2019optinopt}, PlaneCalib~\cite{bartl2020planecalib}, DeepVPCalib~\cite{kocur2021traffic}, and the approach by Revaud et al.~\cite{revaud2021robust}.

OptInOpt~\cite{bartl2019optinopt} and PlaneCalib~\cite{bartl2020planecalib} rely on localizing 2D landmarks using precise 3D CAD models to estimate the camera's focal length and vehicle poses. Notably, these methods were initially developed with the assumption that most vehicles in the BrnoCompSpeed~\cite{sochor2018comprehensive} dataset from the Czech Republic are predominantly manufactured by Skoda. This unique dataset characteristic allowed the original implementations to establish exact 2D-3D correspondences for the keypoints. However, as highlighted in our main manuscript, this assumption isn't realistic and doesn't readily generalize to other regions or countries with diverse car models. In addressing this limitation, we drew inspiration from GSNet~\cite{ke2020gsnet}. Our approach involved classifying each detected car instance into one of four mean shape variations, enabling the establishment of correspondences.
Regarding Revaud et al.'s method~\cite{revaud2021robust}, we used the checkpoint they provided, often referred to as the "learned method" in their work~\cite{revaud2021robust}. This model was exclusively trained using synthetic 3D car models, thus exhibiting limited generalization capabilities.

\section{Statistics}
In our 3D reconstruction pipeline, we use an average of 25 panorama images or 300 perspective images for each intersection. The most computationally intensive step involves SuperGlue feature matching~\cite{sarlin2020superglue}. Here, we match each image with $k = 50$ similar images retrieved using vocabulary tree matching, which results in an average of $15,000$ image pairs. On a single NVIDIA RTX 4090 GPU, this process consumes approximately 20 minutes. It's important to highlight that this process can be parallelized, making it scalable with the number of available GPUs.
When combined with the subsequent COLMAP reconstruction step, the total average runtime for the entire 3D reconstruction workflow amounts to just under 1 hour per scene. Importantly, it's worth noting that the 3D reconstruction only needs to be performed once for each intersection. Following this initial reconstruction, any traffic camera subsequently installed at the same location can be localized with minimal runtime requirements.

\section{More Qualitative Results}

\begin{figure*}[ht]
    \centering
    \includegraphics[width=\textwidth]{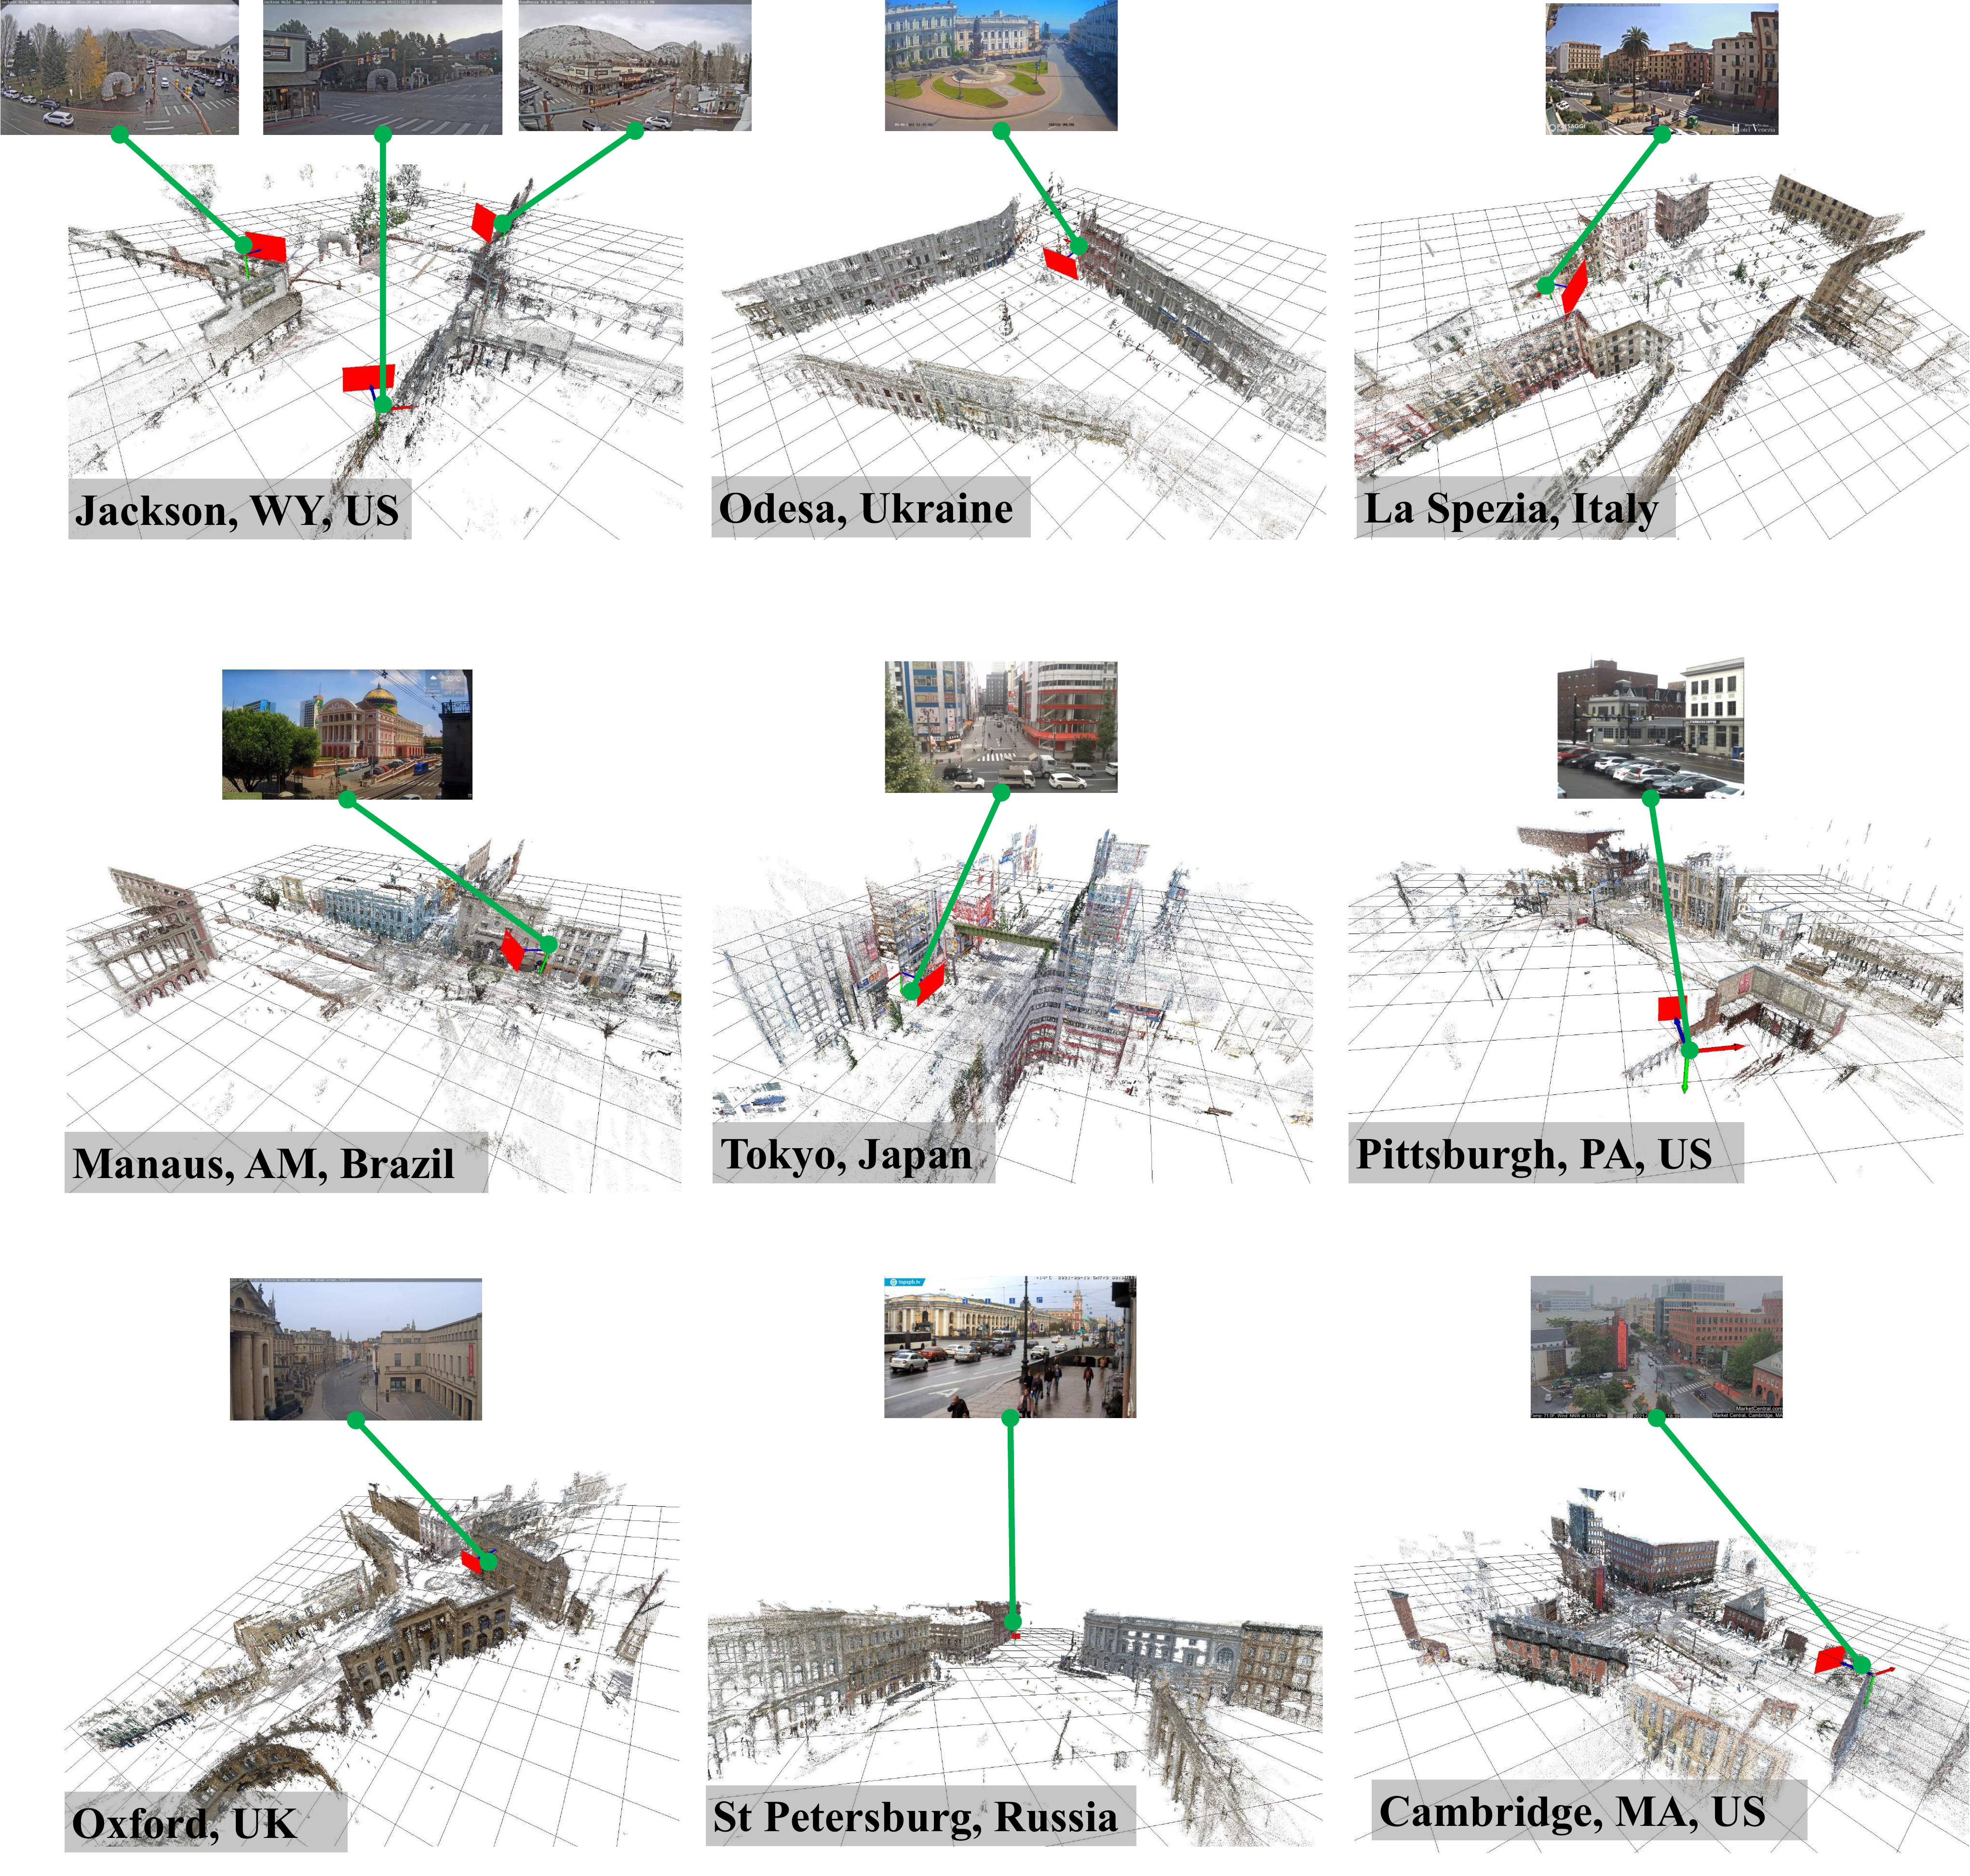}
    \caption{Additional examples demonstrate our method's robustness in reconstructing scenes and localizing cameras spanning various countries and continents (traffic camera visualized in \textcolor{red}{red}).}
    \label{fig:map_loc}
\end{figure*}

Our camera localization method proves versatile across diverse cameras in real-world settings. As depicted in Fig.~\ref{fig:map_loc}, we successfully achieve both accurate 3D scene reconstruction and precise camera localization across different locations spanning multiple countries and continents.
Importantly, our framework's adaptability goes beyond Google Street View, making it versatile for various street-level imagery sources~\cite{BingStreetside, Mapillary}. This enhances scalability, enabling global-scale camera calibration.
